# Supplementary material for: Tackling Interpretability in Audio Classification Networks with Non-negative Matrix Factorization
Source: arXiv:2305.07132 source file (2023-05-11)
Supplement: Supplementary file 1 [file appendix.tex]

\section{Supplementary}

% \subsection{Faithfulness results}
% \begin{table}[!h]
% %\setlength{\tabcolsep}{4pt}
% 	\centering
% %\resizebox{0.5\textwidth}{!}{%	
% 	\begin{tabular}{l c c c} 
% 		\toprule
% 		& & \multicolumn{2}{c}{Faithfulness}\\
% 		\cmidrule[1pt](lr){3-4} 
% 		System & Threshold $\tau$ & mean $\pm$ std & median \\ [0.5ex] 
% 		\midrule
		
% 		\multirow{ 4}{*}{L2I + $\Theta_{\textsc{att}}$} & $\tau=0.9$ & 0.58 $\pm$ 1.32 & 0.21 \\
% 		 & $\tau=0.7$ & 0.87 $\pm$ 1.63 & 0.42 \\
% 		 & $\tau=0.5$ & 1.31 $\pm$ 2.15 & 0.89\\
% 		 & $\tau=0.3$ & 1.65 $\pm$ 2.54 &  1.29\\
% 		\midrule
% 		Random baseline & $\tau=0.3$ & 0.09 $\pm$ 0.76 & 0.00\\
% 		\bottomrule\\
% 	\end{tabular}
% 	%}
% 	\caption{Faithfulness results (absolute drop in logit value) on ESC-50 test--data for different thresholds, $\tau$. We report both, the mean $\pm$ std and the median.}
%     \label{faithfulness_esc50_complete}
% \end{table}

% \begin{figure*}[t]
% \centering
% \includegraphics[width=0.6\textwidth]{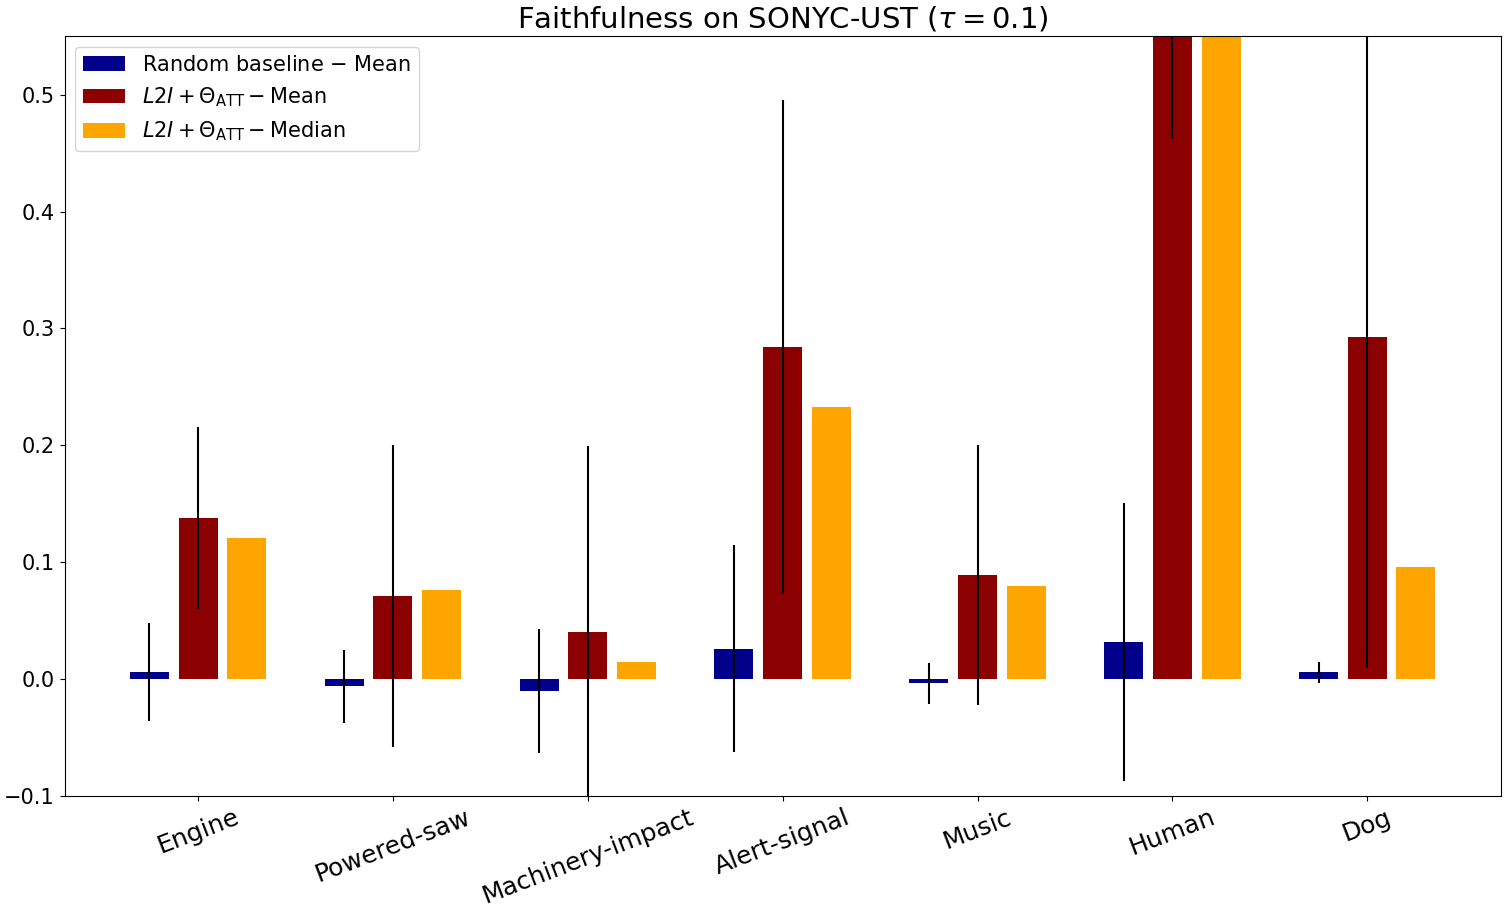}
% \caption{Faithfulness (absolute drop in probability value) results for SONYC-UST dataset arranged class-wise}
% \label{fig_faithfulness_sony_complete}
% \end{figure*}

\subsection{Sparse-NMF implementation details}
\label{supp:sparse-nmf}
The pre-specified dictionary (Step 2 in Algorithm 1) is learnt using Sparse-NMF \cite{le2015sparse}. Specifically, the following optimization problem is solved through multiplicative updates to pre-learn $\Wa$:
\begin{equation}
	\begin{aligned}
		&\text{minimize} & & D(\Va_{\text{train}}|\Wa\Ha) + \mu\|\Ha\|_1\\
			& \text{subject to} & & \Wa \geq 0, \Ha \geq 0,\\
			& & & \|\mathbf{w}_k\|=1,~\forall k.
    \end{aligned}
    \label{eq:sparse-nmf}
\end{equation}
%Training audio files are transformed into log--magnitude spectrogram space for factorization.
Training audio files are converted into log-magnitude spectrogram space for factorization. Here $D(.|.)$ is a divergence cost function. In practice, euclidean distance is used. 

We construct $\Va_{\text{train}}$ differently for each dataset due to their specific properties. For ESC-50,  $\Va_{\text{train}}$ is constructed by concatenating the log--magnitude spectrograms corresponding to each sample in the training data of the cross-validation fold (1600 samples for each fold) and performing joint factorization using Eq. \ref{eq:sparse-nmf}.

SONYC-UST however, is an imbalanced multilabel dataset with very strong presence of background noise. As a result, we process it differently. We first learn $\Wa_{\text{noise}}$, that is, a set of 10 components to model noise using training samples with no positive label. Then, for each class, we randomly select 700 positively-labeled samples from all training data and learn 10 new components (per class) with $\Wa_{\text{noise}}$ held fixed for noise modeling. All $10 \times 8=80$ components are stacked column-wise to build our dictionary $\mathbf{W}$. While this strategy helps us reduce the number of noise-like components in the final dictionary, it does not completely avoid it.

As done in \cite{bisot2017feature}, for computational efficiency, we too average the spectrogram frames over chunks of five. This reduces the size of $\mathbf{X}_{\textrm{train}}$ and saves memory to allow training over more number of samples.

%We first learn 10 components to model noise using training samples with no positive label.

\subsection{Classifier $f$ details}
\label{clf_training}

% MOVE TO Appendix

The architecture we use for $f$ \cite{kumar_wft} has been pretrained on AudioSet. For each dataset, we first fine-tune this network and perform post-hoc interpretations for the resulting trained network. Here we discuss its broad architecture and specific training details used to fine-tune it on our datasets.

It takes as input a log-mel spectrogram. The architecture broadly consists of six convolutional blocks (B1--B6) and one convolutional layer with pooling for final prediction. Most convolutional blocks consist of two sets of conv2D + batch norm + ReLU layers followed by a max pooling layer.

Details of the full architecture can be found in the original reference. For fine-tuning, we modify the architecture of prediction layers. Specifically, we remove the F2 conv layer and add a linear layer after final pooling, the output dimensions of which correspond to the number of classes in our datasets. 

For both the datasets, we do not use any data augmentation. The ADAM optimizer \cite{adam} is used to fine-tune $f$. For ESC-50, we only fine-tune the prediction layers of the network. We train the classifier for 10 epochs on each fold of the dataset with a learning rate of $1 \times 10^{-3}$. 

On SONYC-UST, we fine-tune all the layers in $f$, which leads to higher classifier AUPRC metrics. The classifier is trained for 10 epochs. Here we start with a learning rate of $2 \times 10^{-4}$ and halve it after every 4 epochs. 

%\subsection{Network architectures}

%$\Phi$ consists of 1--2 conv. layers followed by pooling and a FC layer. For LeNet based network, we fix $\mathcal{I}$ as output of $2^{nd}$ conv. layer. For the ResNet18-based network, we fix $\mathcal{I}$ as output of the $3^{rd}$ conv. block (\textit{13th} conv. layer) and middle of the $4^{th}$ conv. block (\textit{15th} conv. layer). Precise architecture details are given in the supplementary.%Architecture of $h$ is fixed as a linear classifier followed by a softmax layer.

%\subsection{Weight tuning} For our experiments we 

%\subsection{Choosing hidden layers}

\subsection{Choosing number of components $K$}
\label{K_choice}

Choice of number of components, $K$, also known as order estimation, is typically data and application dependent. It controls the granularity of the discovered audio spectral patterns. 
Choosing $K$ has also been a long standing problem within the NMF community \cite{tan2012automatic}. Our choice for this parameter was guided by three main factors:
\begin{itemize}
    \item Choices made previously in literature for similar pre-learning of $\mathbf{W}$ \cite{bisot2017feature}, who demonstrated reasonable acoustic scene classification results with a dictionary size of $K=128$. We used this as a reference to guide our choice for number of components.
    
    \item Dataset specific details which include number of classes, samples for each class, variability of recordings etc. For eg. acoustic variability of ESC-50 (larger number of classes), prompted us to use a dictionary of larger size compared to SONYC-UST.
    \item When tracking loss values for different $K$, we observed a plateauing effect for larger dictionary sizes as illustrated in Fig. \ref{fig_loss_vs_K} for ESC-50. 
    
\end{itemize}

\begin{figure}[!ht]
    \centering
    \includegraphics[height=0.28\textwidth, width=0.3\textwidth]{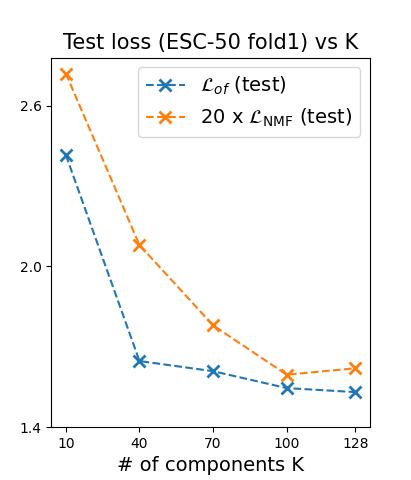}
    \caption{Loss values on ESC50-test data for fold 1 for various dictionary sizes.}
    \label{fig_loss_vs_K}
\end{figure}

%Bisot et al. \cite{bisot2017feature} .  It is worth mentioning that   

\subsection{Other hyperparameters and ablation studies}
\label{hyperparams}

\noindent \textbf{Audio processing parameters}.~ For both the tasks, we perform same audio pre-processing steps. All audio files are sampled at 44.1kHz. STFT is computed with a 1024-pt FFT and 512 sample hop size, which corresponds to about 23ms window size and 11.5ms hop. The log-mel spectrogram is extracted using 128 mel-bands.

\noindent \textbf{Other hyperparameters} We used the same set of hidden layers for both datasets. Specifically, we use the outputs of last three convolutional blocks in $f$, B4, B5 and B6. We also used the same loss hyperparameters $\alpha=10, \beta=0.8$ for both datasets. Models were optimized using ADAM \cite{adam} for 35 epochs on each fold of ESC-50 with learning rate: $2 \times 10^{-4}$ and for 21 epochs on SONYC-UST (learing rate: $5 \times 10^{-4}$). 

Tab. \ref{ablation_hidden_layer} and Tab. \ref{ablation_loss} present ablation studies for loss hyperparameters and choice of hidden layers. The choices in bold indicate our current choices. The metrics and loss values given here are for a single run.

\begin{table}[!t]
\parbox{0.5\columnwidth}{
	\centering
	\resizebox{0.35\columnwidth}{31pt}{
	\begin{tabular}{l c c c} 
		\toprule
		ConvBlocks & $\bmL_{\textrm{NMF}}$ & $\bmL_{of}$ & top-1 \\ [0.5ex] 
		\midrule
		 \textbf{B4+B5+B6} & \textbf{0.079} & \textbf{1.546} & \textbf{65.5} \\
		 B5+B6 & 0.103 & 1.572 & 61.5 \\
		 B6 & 0.118 & 1.698 & 57.8\\
		\bottomrule\\
	\end{tabular}}
	\caption{Hidden layer selection}
    \label{ablation_hidden_layer}
}\hfill
\parbox{0.5\columnwidth}{%
\resizebox{0.5\columnwidth}{!}{
	\begin{tabular}{c c c c c} 
		\toprule
		$\alpha$ & $\beta$ & $\bmL_{\textrm{NMF}}$ & $\bmL_{of}$ & macro-AUPRC \\ [0.5ex] 
		\midrule
		 \textbf{10.0} & \textbf{0.8} & \textbf{0.028} & \textbf{0.386} & \textbf{0.900}\\
		 10.0 & 8.0 & 0.048 & 0.386 & 0.879\\
         10.0 & 0.08 & 0.028 & 0.388 & 0.876\\
         1.0 & 0.8 & 0.045 & 0.375 & 0.921\\
         100.0 & 0.8 & 0.027 & 0.445 & 0.612\\
		\bottomrule\\
	\end{tabular}}
	\caption{Loss hyperparams}
    \label{ablation_loss}}
\vspace{-18pt}
\end{table}

\textbf{Total training time} is around 50 minutes for 1 fold on ESC-50 and 150 minutes for SONYC-UST. Around 30-40\% of the total time is spent on pre-learning $\Wa$ using Sparse-NMF (for both datasets). Networks were trained on a single NVIDIA-K80 GPU.

\subsection{Further discussion on Interpretations}
\label{supp:qualitative}

\subsubsection{Corruption samples ESC-50}
The goal of this experiment is to qualitatively illustrate that our method can generate interpretations on ESC-50 in various noisy situations. For this, we corrupt a given sample from a target class in two ways: (i) With sample from a different class (Overlap experiment), and (ii) Adding high amount of white noise, at 0dB SNR (Noise experiment). The key question that we want the interpretations to offer insight on is: \textit{did the classifier truly make its decision because it "heard" the target class or is it making the decision based on the corruption part of the audio?} The cases where classifier misclassifies are analyzed in Sec. \ref{misclassify}. As already highlighted in Sec. 1, listenable interpretations are not expected to perform source separation for the class of interest, but to confirm if decision corresponds entirely/mostly to target class or not. All examples can be listened to on our companion website \footnote{\url{https://listen2interpret.000webhostapp.com/} \label{footnote 2}}. Since the target and corrupting signals and their classes are already known, we can reinforce the observations drawn by listening to the interpretations through spectrograms (Figs. \ref{fig:spectrograms_1}, \ref{fig:spectrograms_2}).  

\begin{figure}
     \begin{subfigure}[b]{0.4\textwidth}
         \centering
         \includegraphics[width=\textwidth]{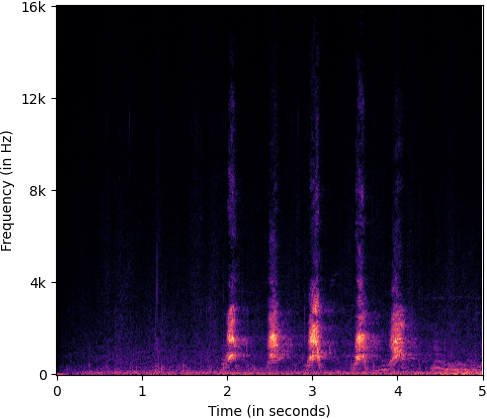}
         \caption{}
         \label{original_target_1}
     \end{subfigure}
     ~
     \begin{subfigure}[b]{0.4\textwidth}
         \includegraphics[width=\textwidth]{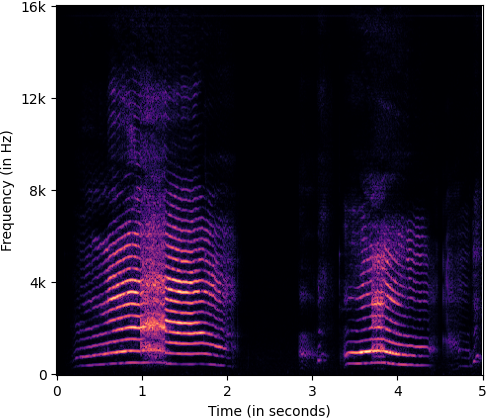}
         \caption{}
         \label{mixer}
     \end{subfigure}
     \\
     \begin{subfigure}[b]{0.4\textwidth}
         \centering
         \includegraphics[width=\textwidth]{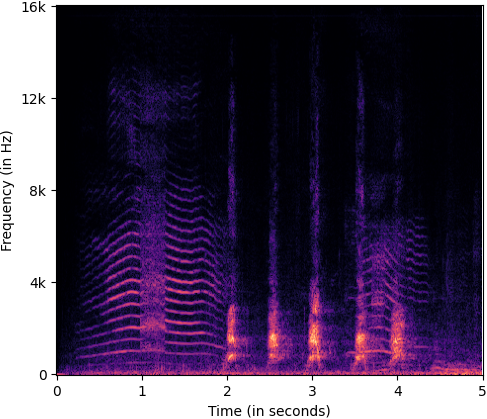}
         \caption{}
         \label{input_audio_1}
     \end{subfigure}
     ~
     \begin{subfigure}[b]{0.4\textwidth}
         \centering
         \includegraphics[width=\textwidth]{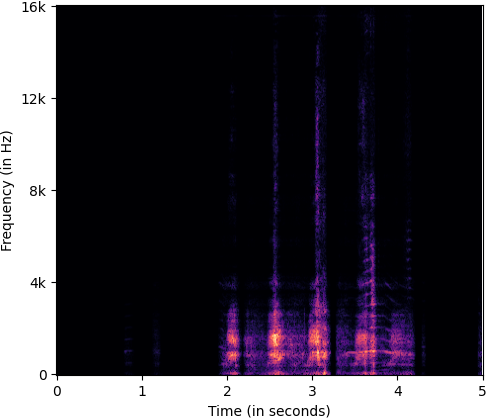}
         \caption{}
         \label{interpretation_1}
     \end{subfigure}
    \vspace{-4pt}
    \caption{Log-magnitude spectrograms of an example from Overlap experiment: (a) Target class ('Dog') original uncorrupted signal (b) Corrupting/Mixing class ('Crying-Baby') signal (c) Corrupted/mixed signal, also the input audio to the classifier (d) Interpretation audio for the predicted class ('Dog'). The interesting observation is that spectrogram of interpretation audio almost entirely consists of parts from target class ('Dog') signal with only a very weak presence of corrupting class ('Crying-Baby') close to the end.}
    \label{fig:spectrograms_1}
\end{figure}

\begin{figure}
     \begin{subfigure}[b]{0.32\textwidth}
         \centering
         \includegraphics[width=\textwidth]{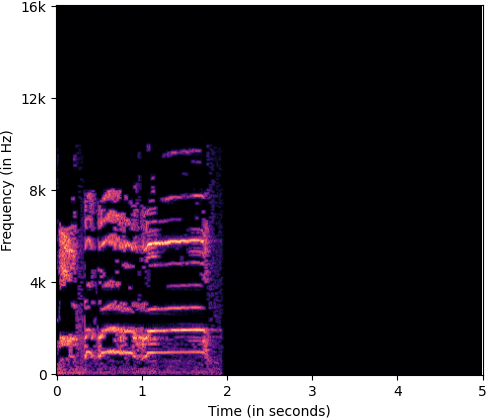}
         \caption{}
         \label{original_target_2}
     \end{subfigure}
     ~
     \begin{subfigure}[b]{0.32\textwidth}
         \centering
         \includegraphics[width=\textwidth]{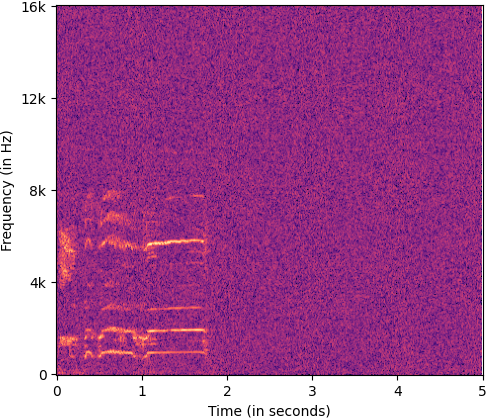}
         \caption{}
         \label{input_audio_2}
     \end{subfigure}
     ~
     \begin{subfigure}[b]{0.32\textwidth}
         \centering
         \includegraphics[width=\textwidth]{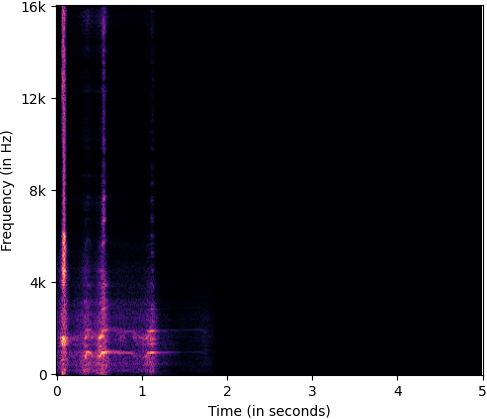}
         \caption{}
         \label{interpretation_2}
     \end{subfigure}
    \vspace{-4pt}
    \caption{Log-magnitude spectrograms of an example from Overlap experiment: (a) Target class ('Rooster') original uncorrupted signal, (b) White noise corrupted signal, also the input audio to the classifier (c) Interpretation audio for the predicted class ('Rooster'). Again, the interpretation audio is almost entirely free of corrupting signal (white noise in this case) and mostly consists of parts of the original target signal. This strongly indicates that the classifier relied on parts of audio corresponding to the target class to make its decision, and not the white noise.  }
    \label{fig:spectrograms_2}
\end{figure} 

\subsubsection{Misclassification samples ESC-50}
\label{misclassify}

When the classifier prediction is incorrect, the interpretations may still provide insight into the classifier's decision by indicating what the classifier ``heard" in the input signal. We give examples for this on the webpage\textsuperscript{\ref{footnote 2}}. For instance, one of the example is of a sample with ground-truth class 'Crying-Baby' misclassified as a 'Car-horn'. Interestingly, the interpretation is acoustically similar to car horns. Please note the importance of \textit{listenable} interpretations that aid such understanding into the audio network's decisions. %The interpretation is interestingly acoustically similar to car horns.

\subsubsection{Coherence in interpretations}
\label{coherence}

We qualitatively analyze the interpretations on SONYC-UST by visualizing relevances generated on the test set. Specifically, we compute the vector $r_{c, x} \in \mathbb{R}^K$ which contains relevances of all components in prediction for class $c$ for sample $x$. The relevance vectors are collected for each test sample $x$ and its predicted class $c$. We then apply a t-SNE \cite{tsne} transformation to 2D for visualization. This is shown in Fig. \ref{tsne_rel}. Each point is colored according to the class for which we generate the interpretation. Interpretations for any single class are coherent and similar to each other. This is to some extent a positive consequence of global weight matrix in $\Theta$. Moreover, globally it can be observed that classes like 'Machinery-impact' and 'Powered-Saw' have similar relevances which are to some extent close to 'Engine'. This is to be expected as these classes are acoustically similar. 'Dog' and 'Music' are also close in this space, likely due to the often periodic nature of barks or beats. %Moreover, globally it can be observed that classes like 'Machinery-impact' and 'Powered-Saw' have similar relevances which are to some extent close to 'Engine'. This is to be expected as these classes are acoustically similar. 'Dog' and 'Music' also have similar relevances, likely due to the often periodic nature of barks or beats.

\begin{figure}[!ht]
    \centering
    \includegraphics[width=0.7\textwidth]{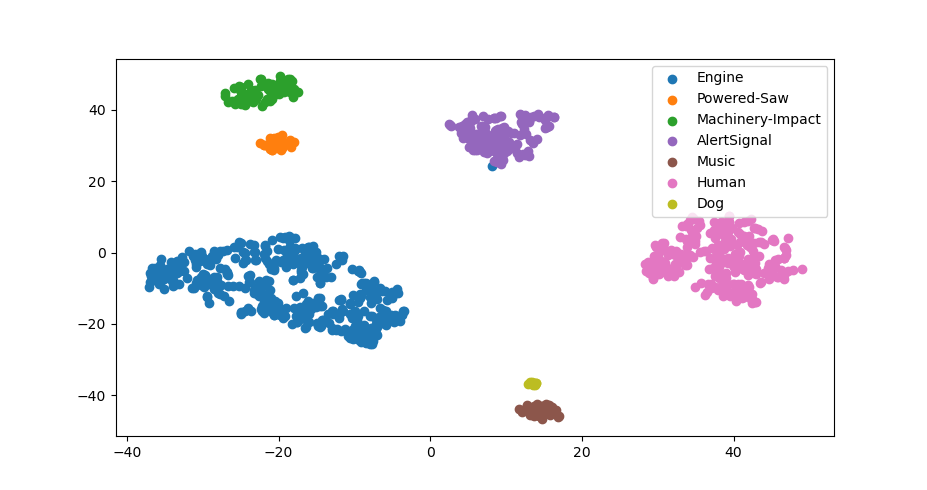}
    \caption{}
    \label{tsne_rel}
\end{figure}

\subsection{Baseline implementations details}
\label{baseline_impl}

\textbf{FLINT}: We implemented it with the help of their official implementation available on GitHub.\footnote{\url{https://github.com/jayneelparekh/FLINT}} For each experiment, we fix their number of attributes $J$ equal to the number of our NMF components $K$. We also choose the same hidden layers for their system as we choose for ours. This baseline is trained for the same number of epochs as us. We use same values for our $\bmL_{\text{NMF}}$ loss weight, $\alpha$, and their $\bmL_{if}$ loss weight $\gamma$. For the other loss hyperparameters, we use their default values and training strategy.
 
\textbf{VIBI}:  We implemented this using their official repository.\footnote{\url{https://github.com/SeojinBang/VIBI}} The key hyperparameters that we set are the input chunk size and their parameter $K$, the number of chunks to use for interpretation. We use a larger chunk size than in their experiments to limit the number of chunks. On ESC-50, we use a chunk size of $32 \times 43$, and on SONYC-UST, a chunk size of $32 \times 86$. This yields 40 chunks for each input on both the datasets. We varied the $K$ from 5 to 20, and report the results with best fidelity. The system was trained for 100 epochs on ESC-50 and 30 epochs on SONYC-UST

\textbf{SLIME}: We primarily relied on implementation from their robustness analysis repository \footnote{\url{https://github.com/saum25/local_exp_robustness}}. The key hyperparameters to balance are the number of chunks vs chunk size. SONYC-UST contains 10 second audio files. This is much longer than 1.6 second audio files for which SLIME was originally demonstrated \cite{slime-1}. Therefore, we divide only on the time-axis to limit the number of chunks. SLIME recommends a chunk size of at least 100ms. They operate on upto 290ms chunk size. We balance these two hyperparameters by dividing our audio files in 20 chunks of 500ms chunk size. We select a maximum of 5 chunks for interpretations and a neighbourhood size of 1000.

\subsection{Subjective evaluation implementation}
\label{sub_eval_details}

The subjective evaluation interface was implemented using webMUSHRA \cite{webMUSHRA}. Prior to voting on the test samples, participants were provided with an instruction page and then a training page with an example to get used to interface, instructions, tune their volume etc. Screenshots of the instruction and training page are given in Fig. \ref{instruction_sub_eval}, Fig. \ref{training_sub_eval} respectively. 

\begin{figure}[!ht]
    \centering
    \includegraphics[width=0.91\textwidth]{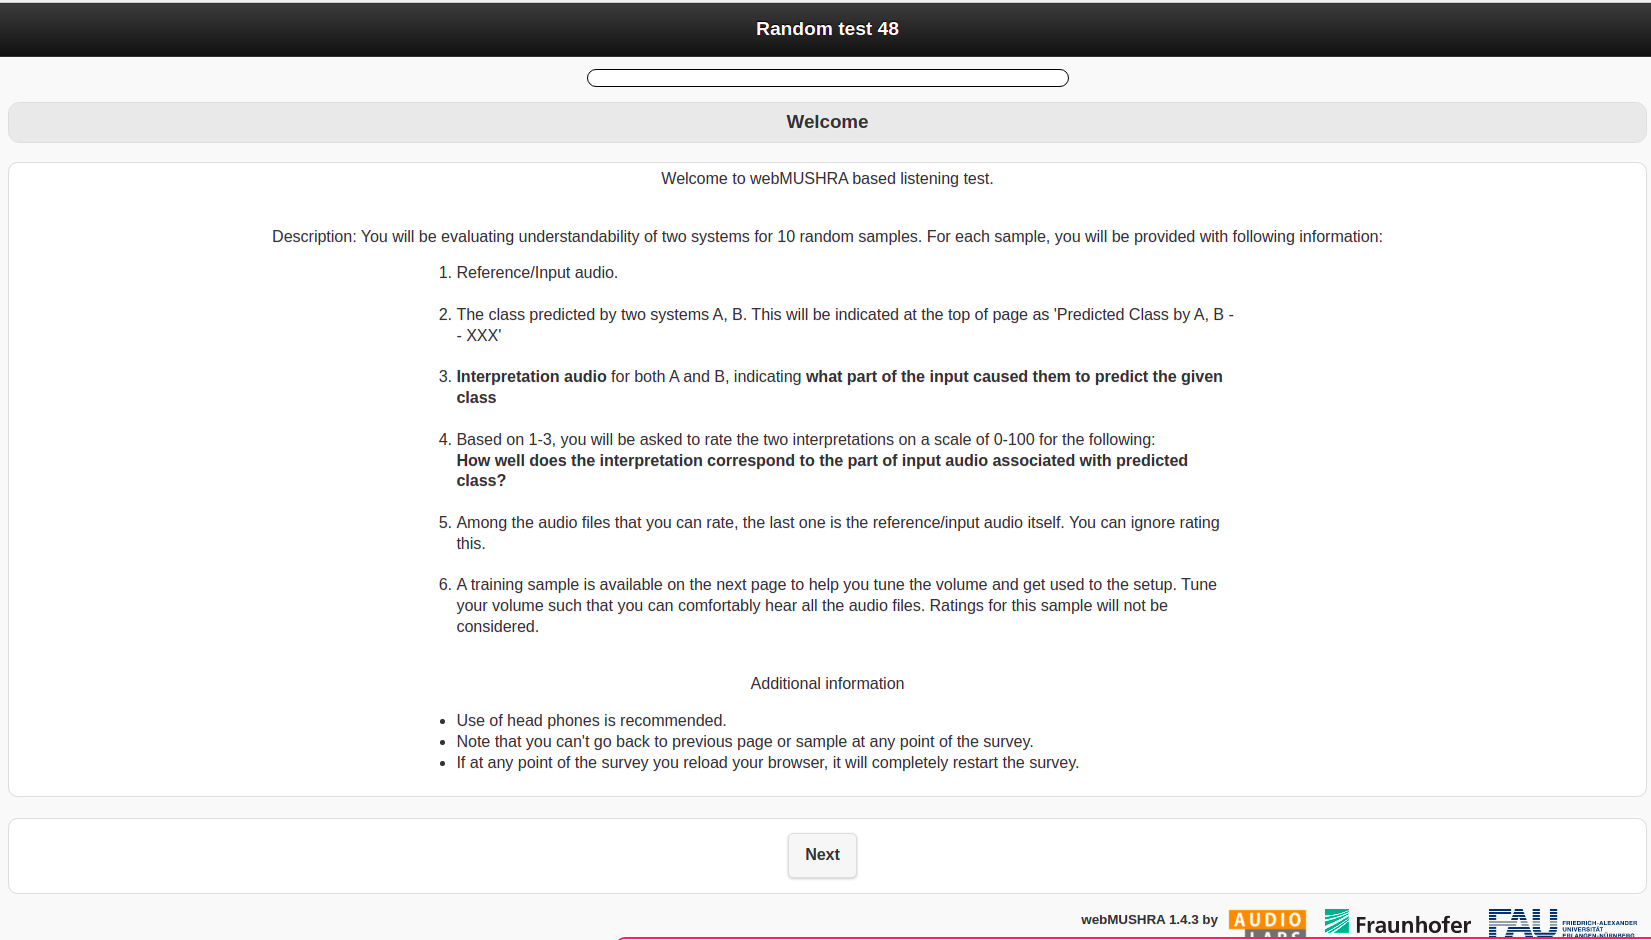}
    \caption{Instructions for the participants at the start of the subjective evaluation}
    \label{instruction_sub_eval}
\end{figure}

\begin{figure}[!ht]
    \centering
    \includegraphics[width=0.91\textwidth]{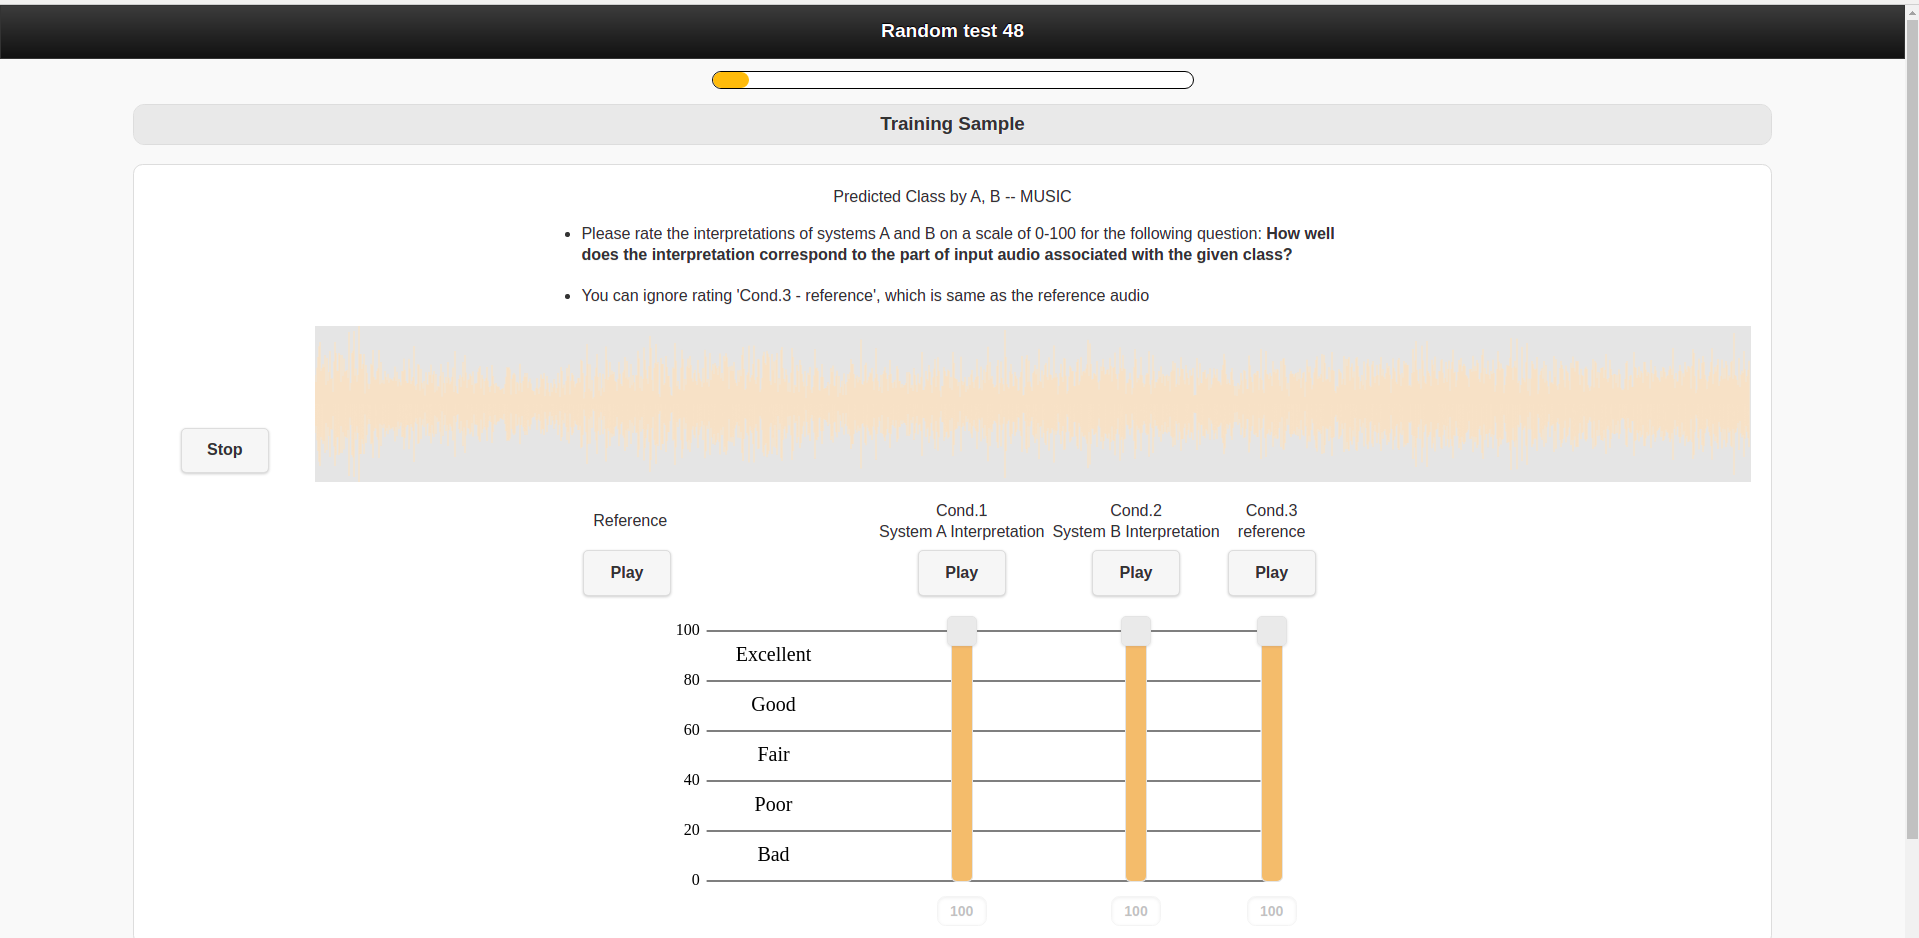}
    \caption{Training page for subjective evaluation that illustrates the interface for scoring for the participants.}
    \label{training_sub_eval}
\end{figure}

\subsection{Limitations and Potential Societal Impacts}

{\bf Limitations.} (1) Tuning the hyperparameters requires some experience with deep architectures and audio. (2) The proposed set of losses are not exhaustive. Modified or additional losses pertaining to other tasks can be imposed on the intermediate encoding.

{\bf Societal Impact.} We expect our method to have positive societal impact by improving understandability of interpretations for audio processing networks. However, this inherently benign technology could be misused when in wrong hands. For example, it can be used to provide misleading interpretations if trained incorrectly (wrong NN architectures, insufficient training examples/training epochs, malicious datasets etc.). Evidently, we expect proper use of the developed methodology, although direct misuse protection mechanisms were not developed in this piece of research, not being the initial goal.

% FLINT text

% Interpretability becoming a frequently raised issue when training and exploiting neural network (NN) architectures, the main expected societal impact of FLINT is improvement of their understandability as well as providing explanations of the decisions made by NNs. Nevertheless, even this intrinsically benevolent machinery can be used for harm when in malicious hands.

% Potential misuse can be expected on two different levels: First, if incorrectly trained (e.g., wrong NN design, insufficient number of training examples and/or or training epochs, in particular for FLINT-f), due to lack of knowledge or on purpose, FLINT can provide misleading interpretations. Second, even a well-trained explainable AI can serve evil purpose in hands of a maliciously destined user.

% Clearly, the authors expect proper use of the developed FLINT methodology, although direct misuseprotection mechanisms were not developed in this piece of research, not being the initial goal

\label{limitations}
